# Supplementary material for: MIMO Multipath-based SLAM for Non-Ideal Reflective Surfaces
Source: arXiv:2404.15375 source file (2024-04-22)
Supplement: Supplementary file 1 [file appendix_DA.tex]

%!TEX root = ../JAIF_2023_V3.tex

\section{Radio Signal Model}
\label{sec:app_signal_model}

In this section we derive the radio signal model described in Section~\ref{sec:signal_model}. 
Usually, specular reflections of radio signals at flat surfaces are modeled by \acp{va} that are mirror images of the \acp{pa} \cite{LeitingerJSAC2015,WitrisalSPM2016,LeitMeyHlaWitTufWin:TWC2019,MenMeyBauWin:JSTSP2019}. 
We start by defining the typical channel impulse response, given for time $n$ and anchor $j$ as
\vspace*{-2mm}
\begin{align}
	h_{\text{c}, n}^{(j)}(\tau) = \rmv\rmv\rmv  \sum_{l = 1}^{{L}_n^{(j)}} {\alpha}_{l,n}^{(j)} \delta\big(\tau\minus {\tau}_{l,n}^{(j)}\big)
\rmv \ist.\\[-7mm]\nn
\end{align}
The first summand describes the \ac{los} component and the sum of ${L}_n^{(j)} \minus 1$ the specular \acp{mpc} with their corresponding complex amplitudes ${\alpha}_{l,n}^{(j)}$ and delays ${\tau}_{l,n}^{(j)}$, respectively. 
In non-ideal radio channels we observe rays to arrive as clusters \cite{SalVal:JSAC1987,KulmerPIMRC2018,PedersenJTAP2018,WenKulWitWym:TWC2021}. The reason for this observation is manifold. Typical examples are non-calibrated antennas, the scattering from a user-body as well as non-ideal reflective surfaces. Fig.~\ref{fig:overview} visualizes these effects, introducing generic impulse responses $h_{\text{ant}, n}^{(j)}(\tau) $ and $h_{\text{surf}, n}^{(j)}(\tau)$. We propose to model the overall impulse response encompassing all considered dispersion effects %(i.e., $h_{\text{ant}\s n}^{(j)}(\tau) $ and $h_{\text{surf}\s n}^{(j)}(\tau) $) 
as
\vspace{-2mm}
\begin{equation}\vspace{-2mm}
	h_{\text{d}, n}^{(j)}(\tau) =	\delta(\tau) + \sum_{i=1}^{S_l^{(j)}} \beta^{(j)}_{l,i,n} 	\delta(\tau -\rmv\rmv\nu^{(j)}_{l,i,n}\big)
\end{equation}
where $\beta^{(j)}_{l,i,n} \in \mathbb{R}$ is a relative dampening variable and $\nu^{(j)}_{l,i,n}$ is the excess delay. The presented model denotes a marked Possion point process \cite{PedersenJTAP2018}. Its statistical properties, i.e, the distribution of $\nu^{(j)}_{l,i,n}$, $\beta^{(j)}_{l,i,n}$, and $S_l^{(j)}$, are discussed in Section~\ref{sec:signal_model} and \ref{sec:system_model} in detail.
We obtain the complex baseband signal received at the $j$th anchor given by the convolution of $h_{\text{d}, n}^{(j)}(\tau)$ and $h_{\text{c}, n}^{(j)}(\tau)$ with the transmitted signal $s(t)$ as \vspace{-2mm}
\begin{align}\label{eq:signal_cont}
\RV{s}_{\text{rx},n}^{(j)} &=   \sum_{l = 1}^{{L}_n^{(j)}} {\alpha}_{l,n}^{(j)} \Big(s(t\minus {\tau}_{l,n}^{(j)} ) \nn\\
&\hspace*{3mm}	+ \sum_{i=1}^{S_l^{(j)}} \beta^{(j)}_{l,i,n} 	s(t \minus {\tau}_{l,n}^{(j)} \minus \rmv\rmv\nu^{(j)}_{l,i,n}) \Big)  +  \rv{\noise{}}_{n}^{(j)}(t)\ist.\\[-7mm]\nn
\end{align}
The second term $\rv{\noise{}}_{n}^{(j)}(t)$ represents an additive white Gaussian noise process with double-sided power spectral density ${N}_{0}^{(j)}/\s 2$.   
%
%The received complex baseband signal at the $j$th \ac{pa} is sampled $N_\text{s}$ times with sampling frequency $ f_{\text{s}} = 1/T_{\text{s}}$ yielding an observation period of $T =  N_{\text{s}} \, T_{\text{s}}$. By stacking the samples, we obtain the discrete-time received signal vector given in \eqref{eq:signal_model_sampled}.
%
%
%
%
%
\section{Data Association}
\label{sec:DA}
This section contains the detailed derivation of the data association-related messages $\varphi^{[p]}_{kl}(b^{(j)}_{l,n})$ and $\nu^{[p]}_{kl}(a^{(j)}_{kl,n})$. Using the measurement evaluation messages in \eqref{eq:message_epsilon1}, \eqref{eq:message_epsilon2} and \eqref{eq:message_epsilon3}, the messages $\underline{\varphi}^{[p]}_{kl}(b^{(j)}_{l,n})$ and $\overline{\varphi}^{[p]}_{ml}(b^{(j)}_{l,n})$ are calculated by
\begin{align}
	\underline{\varphi}^{[p]}_{kl}(b^{(j)}_{l,n}) &= \sum_{\underline{a}^{(j)}_{kl,n} \in \{0,1\}} \varepsilon^{[p]}(\underline{a}^{(j)}_{kl,n})  \underline{\Psi}(\underline{a}^{(j)}_{kl,n},b^{(j)}_{l,n}) \label{eq:app_eq_1}\\
	\overline{\varphi}^{[p]}_{ml}(b^{(j)}_{l,n}) &= \sum_{\overline{a}^{(j)}_{ml,n} \in \{0,1\}} \varepsilon^{[p]}(\overline{a}^{(j)}_{ml,n})  \overline{\Psi}(\overline{a}^{(j)}_{ml,n},b^{(j)}_{l,n})\label{eq:app_eq_2}
\\[-7mm]\nn
\end{align}
for $k \in \{1,\dots,\underline{K}\}$ with $\underline{K} \triangleq K^{(j)}_{n-1}$ and  $m,l  \in \{1,\dots,M^{(j)}_{n}\}$ and are sent from factor node $\underline{\Psi}(\underline{a}^{(j)}_{kl,n},b^{(j)}_{l,n})$ and $\overline{\Psi}(\overline{a}^{(j)}_{ml,n},b^{(j)}_{l,n})$ to variable node $b^{(j)}_{l,n}$, respectively.
By making use of the indicator functions given in \eqref{eq:psi_legacy} and \eqref{eq:psi_new}, respectively, \eqref{eq:app_eq_1} and \eqref{eq:app_eq_2} are also given as
\vspace*{-1mm}
\begin{align}
	\underline{\varphi}^{[p]}_{kl}(b^{(j)}_{l,n}=k) &= \varepsilon^{[p]}(\underline{a}^{(j)}_{kl,n} = 1)  \label{eq:phi_1}\\
	\underline{\varphi}^{[p]}_{kl}(b^{(j)}_{l,n}\neq k) &= \varepsilon^{[p]}(\underline{a}^{(j)}_{kl,n} = 0)  \\
	\overline{\varphi}^{[p]}_{ml}(b^{(j)}_{l,n}= \underline{K} + m) &= \varepsilon^{[p]}(\overline{a}^{(j)}_{ml,n} = 1)  \\
	\overline{\varphi}^{[p]}_{ml}(b^{(j)}_{l,n}\neq \underline{K} + m) &= \varepsilon^{[p]}(\overline{a}^{(j)}_{ml,n} = 0) \label{eq:phi_4}\\[-7mm]\nn
\end{align}
The messages in \eqref{eq:phi_1} - \eqref{eq:phi_4} can be rewritten in the form of
\begin{align}
	\underline{\varphi}^{[p]}_{kl}(b^{(j)}_{l,n}) &= 
	\begin{cases}
		\frac{\varepsilon^{[p]}(\underline{a}^{(j)}_{kl,n} = 1)}{\varepsilon^{[p]}(\underline{a}^{(j)}_{kl,n} = 0)}, &   b^{(j)}_{l,n} = k \\
		1, &  b^{(j)}_{l,n} \neq k
	\end{cases} \label{eq:phi_legacy}\\
	\overline{\varphi}^{[p]}_{ml}(b^{(j)}_{l,n}) &= 
	\begin{cases}
		\frac{\varepsilon^{[p]}(\overline{a}^{(j)}_{ml,n} = 1)}{\varepsilon^{[p]}(\overline{a}^{(j)}_{ml,n} = 0)}, &   b^{(j)}_{l,n} = \underline{K} + m \\
		1, &  b^{(j)}_{l,n} \neq \underline{K} + m.
	\end{cases} \label{eq:phi_new}  
\end{align}

The messages $\underline{\nu}^{[p]}_{kl}(\underline{a}^{(j)}_{kl,n})$ and $\overline{\nu}^{[p]}_{ml}(\overline{a}^{(j)}_{ml,n})$ represent the messages from variable node $\underline{a}^{(j)}_{kl,n}$ to factor node $q( \tilde{\V{x}}_n, {\underline{\V{y}}}^{(j)}_{k,n}, \underline{a}^{(j)}_{kl,n}; \V{z}^{(j)}_{l,n} )$ and from variable node $\overline{a}^{(j)}_{ml,n}$ to factor node $u( \tilde{\V{x}}_n, {\overline{\V{y}}}^{(j)}_{m,n}, \overline{a}^{(j)}_{ml,n}; \V{z}^{(j)}_{l,n} )$, respectively. $\overline{\nu}^{[p]}_{mm}(\overline{a}^{(j)}_{mm,n})$ represents the messages from variable node $\overline{a}^{(j)}_{mm,n}$ to factor node $v( \tilde{\V{x}}_n, {\overline{\V{y}}}^{(j)}_{m,n}, \overline{a}^{(j)}_{mm,n}; \V{z}^{(j)}_{m,n} )$. They are defined as
\begin{align}
\underline{\nu}^{[p]}_{kl}(\underline{a}^{(j)}_{kl,n}) &= \sum_{b^{(j)}_{l,n} = 0}^{K^{(j)}_{n}}  \prod_{\substack{i=1 \\ i\neq k}}^{\underline{K}} \underline{\varphi}^{[p]}_{il}(b^{(j)}_{l,n}) \prod_{m = l}^{M^{(j)}_n}   \overline{\varphi}^{[p]}_{ml}(b^{(j)}_{l,n}) \label{eq:app_eq_3}\\
	\overline{\nu}^{[p]}_{ml}(\overline{a}^{(j)}_{ml,n}) &= \sum_{b^{(j)}_{l,n} = 0}^{K^{(j)}_{n}}  \prod_{i=1}^{\underline{K}} \underline{\varphi}^{[p]}_{il}(b^{(j)}_{l,n}) \prod_{\substack{h=l \\ h\neq m}}^{M^{(j)}_n}  \overline{\varphi}^{[p]}_{hl}(b^{(j)}_{l,n}).\label{eq:app_eq_4}\\[-7mm]\nn
\end{align}
Using the results from \eqref{eq:phi_legacy} and \eqref{eq:phi_new}, \eqref{eq:app_eq_3} and \eqref{eq:app_eq_4} are, respectively, rewritten as
\begin{align}
\underline{\nu}^{[p]}_{kl}(\underline{a}^{(j)}_{kl,n} \rreq 1) =& \prod_{\substack{i=1 \\ i\neq k}}^{\underline{K}} \underline{\varphi}^{[p]}_{il}(b^{(j)}_{l,n} \rreq k) \prod_{m = l}^{M^{(j)}_n}  \overline{\varphi}^{[p]}_{ml}(b^{(j)}_{l,n} \rreq \underline{K} \rrmv + \rrmv k) \nn\\[-4mm]
\text{}\label{eq:nu_final1}\\
\underline{\nu}^{[p]}_{kl}(\underline{a}^{(j)}_{kl,n} = 0) =& \hspace{-5mm} \sum_{\substack{b^{(j)}_{l,n}=0 \\ b^{(j)}_{l,n} \notin \{k,\underline{K} + k\}}}^{K^{(j)}_{n}} \hspace{-2mm} \prod_{\substack{i=1 \\ i\neq k}}^{\underline{K}} \underline{\varphi}^{[p]}_{il}(b^{(j)}_{l,n}) \prod_{m = l}^{M^{(j)}_n}  \overline{\varphi}^{[p]}_{ml}(b^{(j)}_{l,n})\nn \\[-5mm]
\text{}
\end{align}
and 
\begin{align}
\overline{\nu}^{[p]}_{ml}(\overline{a}^{(j)}_{ml,n}  \rreq 1) =& \prod_{i=1}^{\underline{K}} \underline{\varphi}^{[p]}_{il}(b^{(j)}_{l,n}  \rreq  m) \rrmv \rrmv \prod_{\substack{h=l \\ h\neq m}}^{M^{(j)}_n} \rrmv \overline{\varphi}^{[p]}_{hl}(b^{(j)}_{l,n}  \rreq \underline{K}  \rrmv + \rrmv m) \nn\\[-2mm]
\text{}\label{eq:nu_final2}\\
\overline{\nu}^{[p]}_{ml}(\overline{a}^{(j)}_{ml,n} = 0) =&\hspace{-5mm} \sum_{\substack{b^{(j)}_{l,n}=0 \\ b^{(j)}_{l,n} \notin \{m,\underline{K} + m\}}}^{K^{(j)}_{n}} \hspace{-2mm} \prod_{i=1}^{\underline{K}} \underline{\varphi}^{[p]}_{il}(b^{(j)}_{l,n}) \prod_{\substack{h=l \\ h\neq m}}^{M^{(j)}_n}  \overline{\varphi}^{[p]}_{hl}(b^{(j)}_{l,n})\nn \\[-5mm]
\text{}
\end{align}
Note that $\varphi^{[p]}_{kl}(b^{(j)}_{l,n} \rreq 0) = 1$. By normalizing \eqref{eq:nu_final1} by $\underline{\nu}^{[p]}_{kl}(\underline{a}^{(j)}_{kl,n} = 0)$ and \eqref{eq:nu_final2} by $\overline{\nu}^{[p]}_{ml}(\overline{a}^{(j)}_{ml,n} = 0)$, equivalent expressions for \eqref{eq:app_eq_3} and \eqref{eq:app_eq_4} are given as
\begin{align}
&\underline{\nu}^{[p]}_{kl}(\underline{a}^{(j)}_{kl,n}) \nn \\
&= \begin{cases}
		\frac{\prod_{\substack{\scalebox{0.6}{$i=1$}\\ \scalebox{0.6}{$i\neq k$}}}^{\underline{K}} \underline{\varphi}^{[p]}_{il}(b^{(j)}_{l,n} = k) \prod_{m = l}^M  \overline{\varphi}^{[p]}_{ml}(b^{(j)}_{l,n} = \underline{K} + k)}{\sum_{\substack{\hspace{-8mm}\scalebox{0.6}{$b^{(j)}_{l,n}=0$} \\ \scalebox{0.6}{$b^{(j)}_{l,n} \notin \{k,\underline{K} + k\}$}}}^{K^{(j)}_{n}}  \hspace{-4mm} \prod_{\substack{\scalebox{0.6}{$i=1$}\\ \scalebox{0.6}{$i\neq k$}}}^{\underline{K}} \underline{\varphi}^{[p]}_{il}(b^{(j)}_{l,n}) \prod_{m = l}^{M^{(j)}_n}  \overline{\varphi}^{[p]}_{ml}(b^{(j)}_{l,n})}, &   \underline{a}^{(j)}_{kl,n} \rreq 1 \\
		1, & \underline{a}^{(j)}_{kl,n} \rreq 0.
	\end{cases} \label{eq:nu_legacy}\\
&\overline{\nu}^{[p]}_{ml}(\overline{a}^{(j)}_{ml,n})  \nn \\
&\hspace*{0mm}= \begin{cases}
	\hspace*{1mm}	\frac{\prod_{i=1}^{\underline{K}} \underline{\varphi}^{[p]}_{il}(b^{(j)}_{l,n} = m) \prod_{\substack{\scalebox{0.6}{$h=l$}\\ \scalebox{0.6}{$h\neq m$}}}^{M^{(j)}_n}  \overline{\varphi}^{[p]}_{hl}(\bkm)}{\hspace{-2mm} \sum_{\substack{\hspace{-10mm}\scalebox{0.6}{$b^{(j)}_{l,n}=0$} \\ \scalebox{0.6}{$b^{(j)}_{l,n} \notin \{m,\underline{K} + m\}$}}}^{K^{(j)}_n} \hspace{-8mm} \prod_{i=1}^{\underline{K}} \underline{\varphi}^{[p]}_{il}(\scb) \prod_{\substack{\scalebox{0.6}{$h=l$}\\ \scalebox{0.6}{$h\neq m$}}}^{M^{(j)}_n}   \overline{\varphi}^{[p]}_{hl}(\bkm)}, & \hspace*{-3mm} \overline{a}^{(j)}_{ml,n} \rreq 1 \\
		1, & \hspace*{-3mm} \overline{a}^{(j)}_{ml,n} \rreq 0.
	\end{cases} \label{eq:nu_new}  
\end{align}
Finally, by calculating the explicit summations and multiplications in \eqref{eq:nu_legacy} and \eqref{eq:nu_new}, it results in
\begin{align}
&\underline{\nu}^{[p]}_{kl}(\underline{a}^{(j)}_{kl,n}) \nn \\
&\hspace*{3mm}=	\begin{cases}
		\hspace*{-1mm} \frac{1}{1 + \sum_{\substack{\scalebox{0.6}{$i=1$} \\ \scalebox{0.6}{$i\neq k$}}}^{\underline{K}} \underline{\varphi}^{[p]}_{il}(\bi) +  \sum_{m = l}^{M^{(j)}_n}  \overline{\varphi}^{[p]}_{ml}(\bkm)}, &  \rrmv \rrmv \underline{a}^{(j)}_{kl,n} \rreq 1 \\
		1, & \rrmv \rrmv \underline{a}^{(j)}_{kl,n} \rreq 0
	\end{cases} \label{eq:nu_legacy_end}\\[-7mm]\nn
\end{align}
\begin{align}
&\overline{\nu}^{[p]}_{ml}(\overline{a}^{(j)}_{ml,n}) \nn \\ 
&\hspace*{3mm}=\begin{cases}
		\hspace*{-1mm} \frac{1}{1 + \sum_{i=1}^{\underline{K}} \underline{\varphi}^{[p]}_{il}(\bi) +  \sum_{\substack{h=l \\ h\neq m}}^{M^{(j)}_n}  \overline{\varphi}^{[p]}_{hl}(\bkm)}, &  \rrmv \rrmv \overline{a}^{(j)}_{ml,n} \rreq 1\\
		1, & \rrmv \rrmv \overline{a}^{(j)}_{ml,n} \rreq 0.
	\end{cases} \label{eq:nu_new_end}  
\end{align}
